# Supplementary material for: Comparing Meta-GGAs, +U Corrections, and Hybrid Functionals for Polaronic Point Defects in Layered MnO$_2$, NiO$_2$, and KCoO$_2$
Source: arXiv:2404.14317 source file (2024-10-11)
Supplement: Supplementary file 1 [file Polaron_SM.pdf]

# Supplementary Material: Comparing Meta-GGAs, +U Corrections, and Hybrid Functionals for Polaronic Point Defects in Layered $MnO_2$, $NiO_2$, and $KCoO_2$

Raj K. Sah
*Department of Physics, Temple University, Philadelphia, PA 19122*

Michael J. Zdilla and Eric Borguet
*Department of Chemistry, Temple University, Philadelphia, PA 19122*

John P. Perdew
*Department of Physics and Engineering Physics,*
*Tulane University, New Orleans, LA 70118*

**Determination of Hubbard U from Magnetic Moment**

To determine a Hubbard U for some of our calculations, we equated the HSE06+D3 magnetic moment (MM) of ions inside the Wigner-Seitz sphere with the $r^2$SCAN+rVV10+U's MM. First, we relaxed the structure using the HSE06+D3 method and used this structure to calculate the HSE06+D3 MM. We then used the HSE06+D3 structure to do the $r^2$SCAN+rVV10+U calculation, where we slowly varied the U value until $r^2$SCAN+rVV10+U's MM becomes equal to the HSE06+D3's MM. We used smaller bilayer unit cells of transition metal oxides for U determination using this method. We used $MnO_2$, $KMnO_2$, $KNiO_2$, and $CaCoO_2$ to get U values for Mn(IV), Mn(III), Ni(III), and Co(II) ions, respectively. All calculations are performed using the VASP code, where we employed a Gamma-centered Monkhorst-pack grid of size 8 x 8 x 8 and a cut off energy of 400 eV for the plane-wave basis.

First, we used HSE06+D3 with an exact exchange mixing parameter ($\alpha$) of 0.22 to be consistent with Peng et. al.'s work [1]. We have summarized the calculated U value for these ions in Table S1 below.

| | HSE06($\alpha = 0.22$)+D3 MM ($\mu_B$) | $r^2$SCAN+rVV10+U MM ($\mu_B$) | U (eV) |
|---|---|---|---|
| $MnO_2$ | 3.023 | 3.023 | 1.41 |
| $KMnO_2$ | 3.933 | 3.933 | 1.26 |
| $KNiO_2$ | 1.098 | 1.098 | 1.53 |
| $CaCoO_2$ | 2.663 | 2.663 | 0.55 |

TABLE S1. The U value determined by equating the magnetic moments (MM) of HSE06+D3 ($\alpha$ = 0.22) and $r^2$SCAN+rVV10+U, using the HSE06+D3 ($\alpha$ = 0.22) geometry for both functionals.

We could not use this method to determine the U values for Ni(IV) and Co(III) ions using $NiO_2$ and $KCoO_2$ systems because the MM of Ni(IV) and Co(III) ions in $NiO_2$ and $KCoO_2$ is zero, largely independent of the U value, in the $r^2$SCAN+rVV10+U calculation. So, we used the same U values for Ni(IV) and Co(III) as determined for Ni(III) and Co(IV), respectively. We used the U values determined in Table S1, as well as U values from the literature [2], and calculated lattice parameters for $MnO_2$, $NiO_2$, and $CaCoO_2$ unit cells to see how $r^2$SCAN+rVV10+U performs compared to HSE06+D3 with $\alpha$=0.22. The results are summarized in Table S2 below. We see that the lattice constants agree well for $r^2$SCAN+rVV10 and $r^2$SCAN+rVV10+U, but they disagree with HSE06+D3 ($\alpha$=0.22) lattice parameters,

| System | Method | Lattice Parameters (Å) | | | Lattice Angles (Degree) | | |
|---|---|---|---|---|---|---|---|
| | | a | b | c | $\alpha$ | $\beta$ | $\gamma$ |
| $MnO_2$ | $r^2$SCAN+rVV10 | 2.82 | 2.82 | 9.23 | 90 | 90 | 120 |
| | $r^2$SCAN+rVV10+U(1.41 eV) | 2.83 | 2.83 | 9.22 | 90 | 90 | 120 |
| | HSE06($\alpha = 0.22$)+D3 | 2.83 | 2.83 | 9.59 | 90 | 90 | 120 |
| $NiO_2$ | $r^2$SCAN+rVV10 | 2.74 | 2.74 | 8.98 | 90 | 90 | 120 |
| | $r^2$SCAN+rVV10+U(1.53 eV) | 2.73 | 2.73 | 9.00 | 90 | 90 | 120 |
| | HSE06($\alpha = 0.22$)+D3 | 2.72 | 2.72 | 9.25 | 90 | 90 | 120 |
| $KCoO_2$ | $r^2$SCAN+rVV10 | 2.89 | 2.89 | 11.64 | 90 | 90 | 120 |
| | $r^2$SCAN+rVV10+U(0.55 eV) | 2.89 | 2.89 | 11.65 | 90 | 90 | 120 |
| | HSE06($\alpha = 0.22$)+D3 | 2.86 | 2.86 | 11.21 | 90 | 90 | 120 |

TABLE S2. Lattice parameters and lattice angles comparison for $r^2$SCAN+rVV10, $r^2$SCAN+rVV10+U and HSE06($\alpha = 0.22$)+D3 methods for the systems $MnO_2$, $NiO_2$ and $KCoO_2$ .

especially the c parameter. Probably this is because the D3 parameters were determined for HSE06 at $\alpha = 0.25$, not 0.22.This motivated us to go back to full HSE06.

| | HSE06($\alpha = 0.25$)+D3 MM ($\mu_B$) | $r^2$SCAN+rVV10+U MM ($\mu_B$) | U (eV) |
|---|---|---|---|
| $MnO_2$ | 3.036 | 3.036 | 1.71 |
| $KMnO_2$ | 3.947 | 3.947 | 1.58 |
| $KNiO_2$ | 1.163 | 1.163 | 2.06 |
| $CaCoO_2$ | 2.683 | 2.683 | 0.91 |

TABLE S3. The U value determined by equating the magnetic moments (MM) of HSE06+D3 ($\alpha$ = 0.25) and $r^2$SCAN+rVV10+U, using the HSE06+D3 ($\alpha = 0.25$) geometry for both functionals.

As above, we again determined U values by comparing the MM of $r^2$SCAN+rVV10+U with the full HSE06+D3 ($\alpha$=0.25 ) functional. Table S3 below summarizes the result. The U values determined in the Table S3 are closer to the values in the literature, where optimal values for Mn, Ni, and Co ions for $r^2$SCAN are 1.8 eV, 2.1 eV, and 1.8 eV, respectively [2]. The difference in oxidation states of ions could be the cause of the discrepancy. We used the above U values for the $r^2$SCAN+rVV10+U functional and again compared the lattice parameters. The results are summarized in Table S4 below.

| System | Method | Lattice Parameters (Å) | | | Lattice Angles (Degree) | | |
|---|---|---|---|---|---|---|---|
| | | a | b | c | $\alpha$ | $\beta$ | $\gamma$ |
| $MnO_2$ | $r^2$SCAN+rVV10 | 2.82 | 2.82 | 9.23 | 90 | 90 | 120 |
| | $r^2$SCAN+rVV10+U(1.71 eV) | 2.84 | 2.84 | 9.11 | 90 | 90 | 120 |
| | HSE06($\alpha = 0.25$)+D3 | 2.82 | 2.82 | 9.25 | 90 | 90 | 120 |
| $NiO_2$ | $r^2$SCAN+rVV10 | 2.74 | 2.74 | 8.98 | 90 | 90 | 120 |
| | $r^2$SCAN+rVV10+U(2.06 eV) | 2.73 | 2.73 | 8.98 | 90 | 90 | 120 |
| | HSE06($\alpha = 0.25$)+D3 | 2.73 | 2.73 | 9.03 | 90 | 90 | 120 |
| $KCoO_2$ | $r^2$SCAN+rVV10 | 2.89 | 2.89 | 11.64 | 90 | 90 | 120 |
| | $r^2$SCAN+rVV10+U(0.91 eV) | 2.89 | 2.89 | 11.65 | 90 | 90 | 120 |
| | HSE06($\alpha = 0.25$)+D3 | 2.87 | 2.87 | 11.61 | 90 | 90 | 120 |

TABLE S4. Lattice parameters and lattice angles comparison for $r^2$SCAN+rVV10, $r^2$SCAN+rVV10+U and HSE06($\alpha = 0.25$)+D3 methods for the systems $MnO_2$, $NiO_2$ and $KCoO_2$.

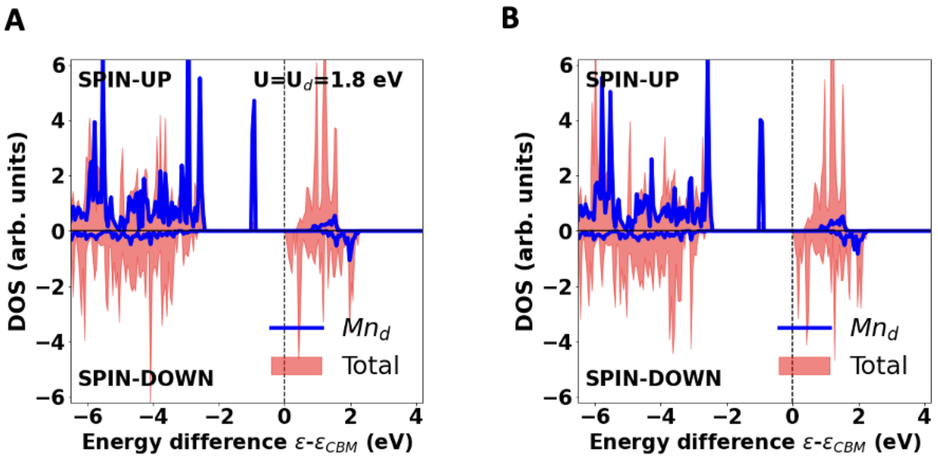


FIG. S1. Spin-resolved density of states per atom using $r^2$SCAN+rVV10+U+$U_d$ (with U=$U_d$=1.8 eV) geometry in a single K-intercalated $MnO_2$ using (A) HSE06 (with $\alpha$=0.22) and (B) HSE06 (with $\alpha$=0.22)+D3.

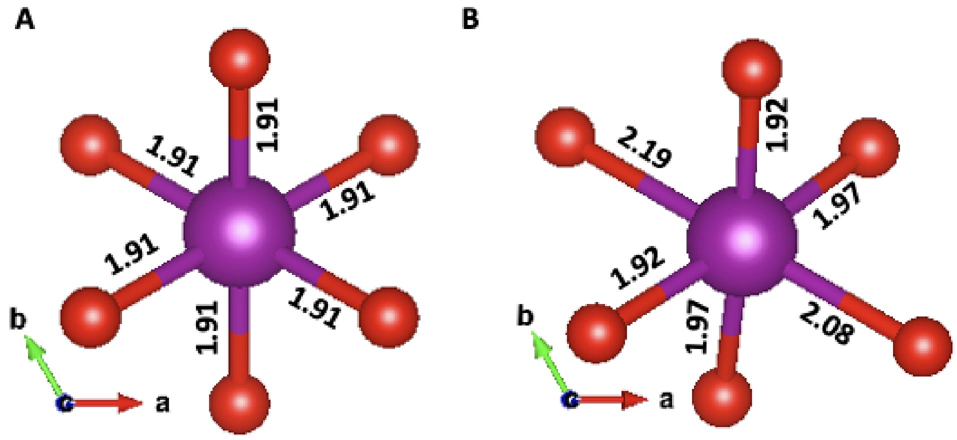


FIG. S2. (**A**) Mn(IV) - O bond lengths in pristine $MnO_2$ and **(B)** defect Mn(III) - O bond lengths in a K-intercalated $MnO_2$ ($K_{0.03}MnO_2$) calculated using the $r^2$SCAN+rVV10+U+$U_d$ (with U=$U_d$=1.8 eV) functional, showing the Jahn-Teller symmetry breaking of the MnO6 octahedron. All lengths are in angstrom units. The red balls represent O ions and purple Mn ions. In the pristine materials, the three $t_{2g}$ $(d_{xy}, d_{yz}, d_{zx})$ space orbitals are equally populated, and the two $e_g$ $(d_{x^2-y^2}, d_{z^2})$ spatial orbitals (whose lobes point from the metal cation to the 6 oxygens on the corners of the octahedron) are empty.

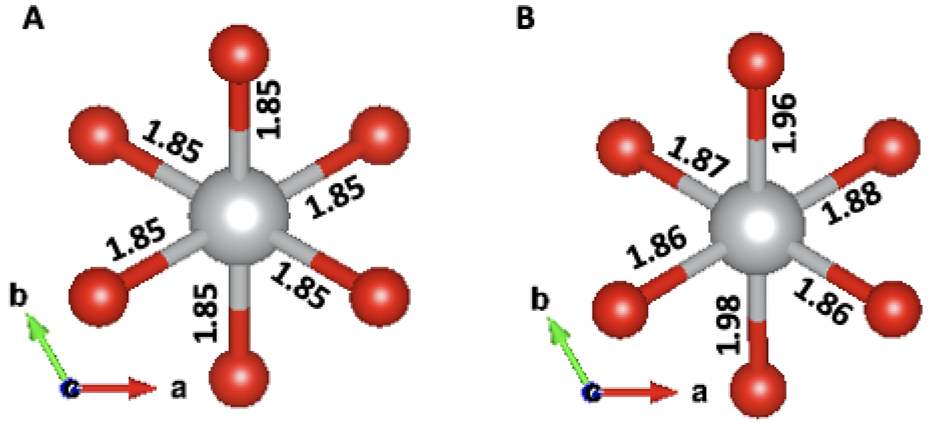


FIG. S3. (**A**) Ni(IV) - O bond lengths in pristine $NiO_2$ and **(B)** defect Ni(III) - O bond lengths in a K-intercalated $MnO_2$ ($K_{0.03}NiO_2$) calculated using the $r^2$SCAN+rVV10+U+$U_d$ (with U=$U_d$=2.1 eV) functional, showing the Jahn-Teller symmetry breaking of the NiO6 octahedron. All lengths are in angstrom units. The red balls represent O ions and silver Ni ions. In the pristine materials, the three $t_{2g}$ $(d_{xy}, d_{yz}, d_{zx})$ space orbitals are equally populated, and the two $e_g$ $(d_{x^2-y^2}, d_{z^2})$ spatial orbitals (whose lobes point from the metal cation to the 6 oxygens on the corners of the octahedron) are empty.

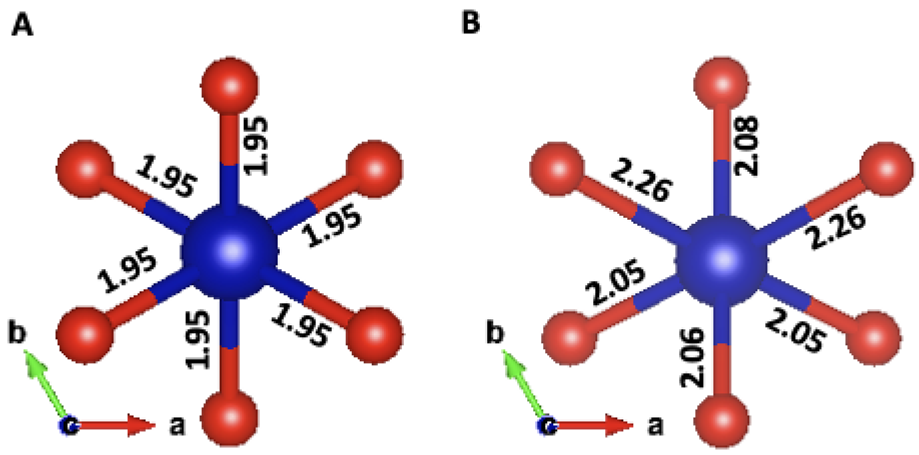


FIG. S4. (**A**) Co(III) - O bond lengths in pristine $KCoO_2$ and **(B)** defect Co(II) - O bond lengths in a K-intercalated $KCoO_2$ ($K_{1.03}CoO_2$) calculated using the $r^2$SCAN+rVV10+U+$U_d$ (with U=$U_d$=1.8 eV) functional, showing the Jahn-Teller symmetry breaking of the CoO6 octahedron. All lengths are in angstrom units. The red balls represent O ions and blue Co ions. In the pristine materials, the three $t_{2g}$ ($d_{xy}, d_{yz}, d_{zx}$) space orbitals are equally populated, and the two $e_g$ ($d_{x^2-y^2}, d_{z^2}$) spatial orbitals (whose lobes point from the metal cation to the 6 oxygens on the corners of the octahedron) are empty.

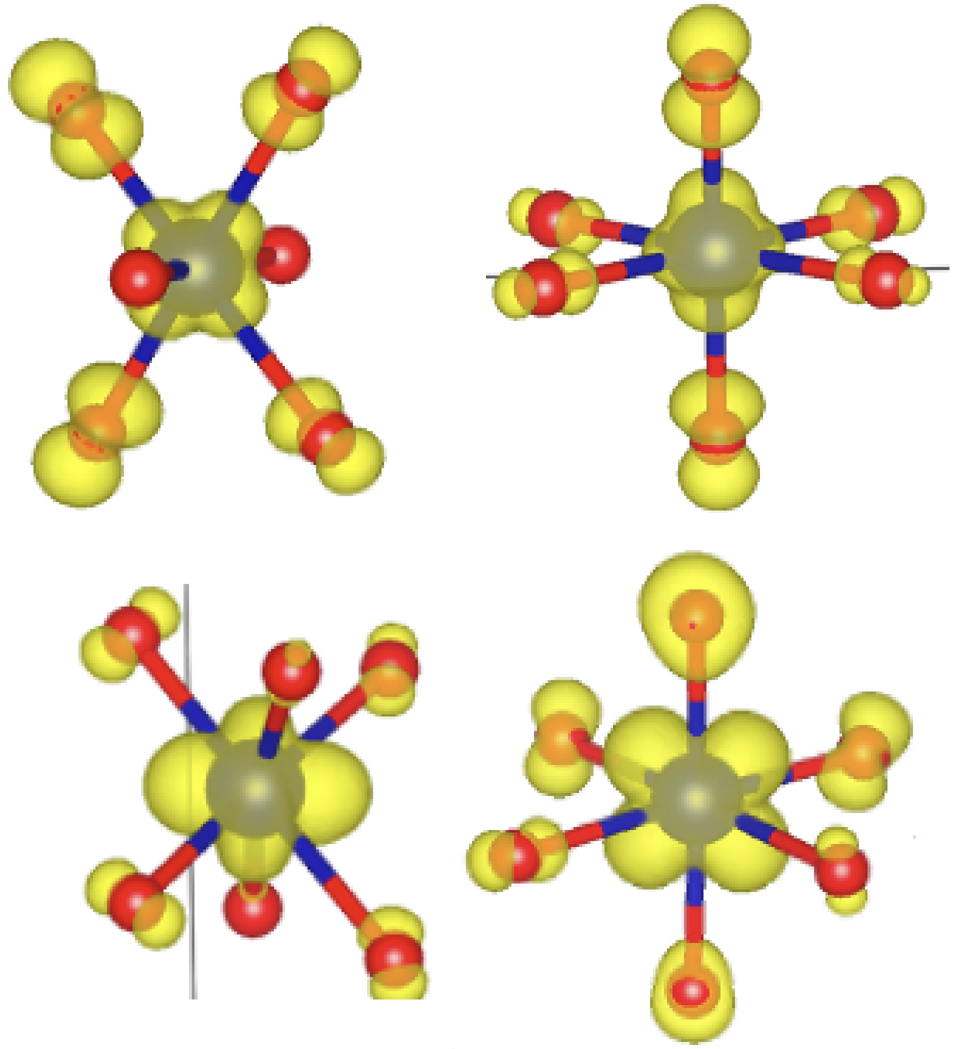

FIG. S5. $r^2$SCAN + rVV10 + U + $U_d$ ($U = U_d = 1.8$ eV) based total charge density plots of four localized orbitals in the band gap region of $K_{1.03}CoO_2$ around the defect Co(II) ion . The plots in the upper panel correspond to the two highest occupied orbitals in the spin up channel and clearly show them to be the $e_g$ orbitals. The lower panel corresponds to the two highest occupied orbitals in the spin down channel and shows them to be the $t_{2g}$ orbitals.
